# Supplementary material for: On the Stability of Nonlinear Receding Horizon Control: A Geometric Perspective
Source: arXiv:2103.15010 source file (2024-01-25)
Supplement: Supplementary file 2 [file cdc_appendix.tex]

In view of \Cref{lem:comparison}, to obtain a bound on $\Vtil(s)$ it suffices to bound  $\Vjacst(s) :=\inf_{\ubar_{[s,T]}} \Jlin_{T-s}(\cdot, ~ \xtil(s), \util_{[s,T]})$. Moreover, we can bound $\Vjacst(s)$ by bounding $\Jlin_{T-s}(\ubar_{[s,T]};~ \xtil(t), \util_{[s,T]})$ for any (possibly suboptimal) control $\ubar_{[s,T]}$; for simplicity, let us drop the ${[s,T]}$-subscript going forward. We select $\ubar(t) = \ubar_1(t) + \ubar_2(t)$, where $\ubar_1(t)$ satisfies $\Btil(t) \ubar_1(t) =- \tilde{d}(t)$, and where $\ubar_2$ witnesses $\gamma$-stabilizability at time $s$ as in \Cref{asm:stabilizable}.

With this choice of $\ubar(t)$ the dynamics of $\xbar(t)$ in $\Jlin_{T-s}$  are $\tfrac{\rmd}{\rmd t} \xbar(t) = \Atil(t)\xbar(t) + \Btil(t)\ubar(t) + \tilde{d}(t) = \Atil(t)\xbar(t) + \Btil \bar{u}_2(t)$, and, writing out $\Jlin_{T-s}$ explicitly, we obtain
\begin{align} 
\Vjacst(s) \le \textstyle \int_{t=s}^T (Q(\xbar(t)) + R(\ubar(t))\rmd t + V(\xbar(T)).
\end{align}
By the elementary bound $\|\ubar(t)\|^2 \le 2\|\ubar_1(t)\|^2 + 2\|\bar{u}_2(t)\|^2$, the following holds for constant $c = \max\{\beta_V,2\beta_R,\beta_Q\}$,
\begin{align}\textstyle
&\Vjacst(s)\textstyle\le   2\beta_R \int_{t=s}^T \|\ubar_1(t)\|^2 \dt \label{eq:P_line_one}\\
&\quad+c \left(\textstyle\int_{t=s}^T (\|\xbar(t)\|^2 + \|\ubar(t)\|^2)\rmd t + \|\xbar(T)\|^2\right). \label{eq:P_line_two}
\end{align}
To bound \eqref{eq:P_line_two}, we observe that $\ddt \xbar(t) = \Atil(t)\xbar(t) + \Btil(t)\ubar(t) + \tilde{d}(t) = \Atil(t)\xbar(t) + \Btil(t)\bar{u}_2(t)$, which corresponds to the $\hat{x}(t)$ dynamics in the definion of $\gamma$-stabilizability; thus, \eqref{eq:P_line_two} is at most $c \cdot \gamma \|\xtil(s)\|^2$. 

To bound \eqref{eq:P_line_one}, we use \eqref{asm:linearizable_bound} to bound $ \|\ubar_1(t)\|^2 \le  2L_x^2\|\xtil(t)\|^2 + 2 L_u^2\|\util(t)\|^2 \le 2c'(Q(\xtil(t)) +  R(\util(t))/\beta_R$, where $c' =  \beta_R\max\{\frac{L_x^2}{\alpha_Q},\frac{ L_u^2}{\alpha_R})$. Hence,  in view of \Cref{lem:comparison}, and the principle of optimality:
\begin{align*}
& 2 \beta_R\textstyle\int_{t=s}^T \|\bar{u}_1(t)\|^2 \dt \le  4c'\beta_R \textstyle\int_{t=s}^T (Q(\xtil(t)) +  R(\util(t))\dt \\
&\quad \le  4c' \beta_R \Vtil(s)  \le 4c'\beta_R(\Vjacst(s)  + \tfrac{\epsilon^2}{2\alpha_R})
\end{align*}
Putting the bounds together and rearranging:
\begin{align*}
(1-   4 \beta_R c' )\Vjacst(s) \le c \cdot \gamma \|\xtil(s)\|^2 + \tfrac{2 c'\beta_R}{ \alpha_R} \epsilon^2
\end{align*}
Under \Cref{asm:linearizable_bound}, we have $4\beta_R c'\le 1/2$, so that
\begin{align}
\Vjacst(s) \le 2c\cdot \gamma \|\xtil(s)\|^2 + 4 c'\beta_R \epsilon^2/\alpha_R.
\end{align}
We recognize $2c\gamma \le \calC_1$, and $\tfrac{4 c' \beta_R}{\alpha_R} = \calC_2 - \frac{1}{2\alpha_R}$, and invoke \Cref{lem:comparison} to obtain the desired bound. \qedd
